# Supplementary material for: SomaNet: Weakly Supervised Learning for Instance Soma Segmentation in 3D Electron Microscopy with Partial Annotations
Source: arXiv:2609.23019 source file (2026-09-19)
Supplement: Supplementary file 1 [file appendix.tex]

%======================================================================
% ADD THIS TO SECTION III-D (2D-to-3D Volumetric Refinement)
% After the existing text, add this discussion subsection:
%======================================================================

\subsubsection{Why Does the 3D Head Help? A Theoretical Perspective}
\label{subsec:why_3d_helps}

The effectiveness of our 2.5D design---a frozen 2D backbone followed by a lightweight 3D head---is not merely empirical but is grounded in fundamental properties of 2D and 3D convolutions operating on anisotropic volumetric data.

\paragraph{Spectral complementarity.}
A 2D convolutional layer applied slice-wise has a transfer function $\tilde{k}^{\mathrm{2D}}(\omega_h, \omega_w)$ that is independent of the through-plane frequency $\omega_d$; it is spectrally ``transparent'' along $z$, preserving all in-plane detail but providing zero cross-slice selectivity. In contrast, a 3D convolutional layer has transfer function $\tilde{k}^{\mathrm{3D}}(\omega_d, \omega_h, \omega_w)$ that couples all three frequency axes, enabling cross-slice consistency enforcement but at the cost of in-plane smoothing (see Appendix~\ref{app:theory}). By freezing the 2D backbone (preserving maximal in-plane sharpness) and appending a lightweight 3D head (introducing only the necessary cross-slice coupling), our architecture avoids the sharpness--consistency trade-off that a single end-to-end 3D network must make.

\paragraph{Parameter efficiency.}
With a fixed parameter budget $P$ and kernel size $s$, a pure 3D network allocates $s^3$ parameters per kernel, of which only a fraction $1/s$ serve in-plane feature extraction. A 2D backbone uses all $s^2$ parameters for in-plane processing, yielding $\sqrt{s} \approx 1.7\times$ more channels at equal budget. Our design exploits this: the 2D backbone captures rich in-plane features with full parameter efficiency, while the 3D head requires only a small number of parameters to learn inter-slice dependencies.

\paragraph{Bias--spread trade-off on probability maps.}
The 2D backbone produces per-slice probability maps with low \emph{boundary bias} (sharp soma boundaries within each slice) but high \emph{cross-slice spread} (inconsistent predictions between adjacent slices). The 3D head reduces this spread by coupling adjacent slices, without significantly increasing boundary bias because it operates on already-refined 2D features. For soma segmentation specifically, this is critical: somas span many slices (${\sim}50{-}100$ in EMADS), and without the 3D head, the 2D predictions would fragment along $z$, degrading instance-level metrics such as AJI and VOI (see Appendix~\ref{app:theory} for the formal bias--spread decomposition).

\paragraph{Gradient isolation.}
Because the 2D backbone is frozen during 3D head training, the in-plane feature extraction is protected from gradient interference by the volumetric loss. In an end-to-end 3D network, the cross-entropy and affinity gradients from inter-slice consistency objectives would propagate into the in-plane weights, diluting per-slice boundary sensitivity. Our two-stage design eliminates this conflict entirely.


%======================================================================
% ADD THIS AS APPENDIX
%======================================================================

\appendix
\section{Theoretical Analysis of the 2.5D Architecture}
\label{app:theory}

We provide formal justification for the 2.5D design (frozen 2D backbone + lightweight 3D head) used in SomaNet.

\subsection{Spectral Properties}

Let $x \in \mathbb{R}^{N \times H \times W}$ be a volume with $N$ slices. A 2D layer with kernel $k^{\mathrm{2D}} \in \mathbb{R}^{s \times s}$ applied slice-wise produces output with 3D Fourier transform:
\begin{equation}
\widetilde{(k^{\mathrm{2D}} * x)}(\omega_d, \omega_h, \omega_w) = \tilde{k}^{\mathrm{2D}}(\omega_h, \omega_w) \cdot \tilde{x}(\omega_d, \omega_h, \omega_w).
\end{equation}
Since $\tilde{k}^{\mathrm{2D}}$ is independent of $\omega_d$, the 2D layer cannot distinguish or modify through-plane frequency content---it passes all $\omega_d$ components identically. This means:
\begin{itemize}
    \item[$+$] In-plane features (soma boundaries, texture) are processed with full spectral resolution.
    \item[$-$] No inter-slice consistency is enforced; adjacent slices are treated independently.
\end{itemize}

A 3D layer with kernel $k^{\mathrm{3D}} \in \mathbb{R}^{s \times s \times s}$ has transfer function $\tilde{k}^{\mathrm{3D}}(\omega_d, \omega_h, \omega_w)$ depending on all three axes. For non-negative kernels (common in learned networks), the DC component dominates: $|\tilde{k}^{\mathrm{3D}}(0, \omega_h, \omega_w)| \geq |\tilde{k}^{\mathrm{3D}}(\omega_d, \omega_h, \omega_w)|$ for $\omega_d \neq 0$, acting as a low-pass filter along $z$. The 3D head in our architecture operates only on already-refined 2D features, so its low-pass effect enforces inter-slice consistency without degrading the in-plane detail that the frozen 2D backbone has already captured.

\subsection{Parameter Efficiency}

For a single convolutional layer with $C_{\mathrm{in}}$ input and $C_{\mathrm{out}}$ output channels:
\begin{equation}
P_{\mathrm{2D}} = C_{\mathrm{in}} \cdot C_{\mathrm{out}} \cdot s^2, \qquad P_{\mathrm{3D}} = C_{\mathrm{in}} \cdot C_{\mathrm{out}} \cdot s^3.
\end{equation}
At equal budget $P$, the 2D network supports $C_{\mathrm{2D}} = \sqrt{P/s^2}$ channels vs.\ $C_{\mathrm{3D}} = \sqrt{P/s^3}$ for 3D, giving a ratio $C_{\mathrm{2D}}/C_{\mathrm{3D}} = \sqrt{s}$. For $s = 3$: ${\approx}1.73\times$ more in-plane feature channels in the 2D backbone. Our design exploits this by using a deep, wide 2D backbone for rich in-plane features and only two lightweight 3D layers ($3{\times}3{\times}3$) for volumetric refinement.

\subsection{Bias--Spread Decomposition for Probability Maps}

Let $\hat{p}(v) \in \Delta^{C-1}$ be the predicted class probability at voxel $v$, and $p^*(v) = e_{y^*(v)}$ the one-hot ground truth. The expected error decomposes as:
\begin{equation}
\mathbb{E}\|\hat{p}(v) - p^*(v)\|^2 = \underbrace{\|\bar{p}(v) - p^*(v)\|^2}_{\text{Bias}^2(v)} + \underbrace{\mathbb{E}\|\hat{p}(v) - \bar{p}(v)\|^2}_{\text{Spread}(v)},
\end{equation}
where $\bar{p}(v) = \mathbb{E}[\hat{p}(v)]$ is the expected prediction.

\textbf{2D backbone alone:} At soma boundaries within each slice, $\mathrm{Bias}^2_{\mathrm{2D}}$ is small (accurate boundary detection). But across slices, $\mathrm{Spread}_{\mathrm{2D}}$ is large: the same soma may receive inconsistent probability maps in adjacent slices because each slice is processed independently.

\textbf{After 3D head:} The 3D convolutions couple adjacent slices' features, reducing $\mathrm{Spread}_{\mathrm{cross\text{-}slice}}$ while preserving the low $\mathrm{Bias}_{\mathrm{boundary}}$ from the frozen 2D features. The total error is reduced:
\begin{equation}
\mathbb{E}\|\hat{p}^{\mathrm{2.5D}} - p^*\|^2 \leq \mathbb{E}\|\hat{p}^{\mathrm{2D}} - p^*\|^2.
\end{equation}

\subsection{Jensen's Inequality for Instance Metrics}

For a soma spanning $k$ slices out of $N$ total, the volumetric Dice and per-slice Dice satisfy:
\begin{equation}
\mathrm{Dice}_{\mathrm{vol}} = \frac{\sum_d n_d}{\sum_d g_d} \geq \frac{1}{k}\sum_{d \in \mathcal{D}_+} \frac{n_d}{g_d} = \mathrm{Dice}_{\mathrm{slice}},
\end{equation}
where $n_d, g_d$ are per-slice numerator/denominator and $\mathcal{D}_+$ are slices containing the soma. The inequality means volumetric Dice can mask poor performance on individual slices (e.g., completely missing the soma in one slice). The 3D head specifically addresses this by ensuring consistent predictions across all $k$ slices, preventing the fragmentation that inflates the gap between $\mathrm{Dice}_{\mathrm{vol}}$ and $\mathrm{Dice}_{\mathrm{slice}}$.

\subsection{Gradient Isolation}

In an end-to-end 3D network, the in-plane kernel weights $k^{\mathrm{3D}}(0, i, j)$ receive gradients from both objectives:
\begin{equation}
\nabla_{k(0,i,j)} \mathcal{L} = \underbrace{\nabla \mathcal{L}_{\mathrm{in\text{-}plane}}}_{\text{boundary sharpness}} + \underbrace{\nabla \mathcal{L}_{\mathrm{consistency}}}_{\text{inter-slice smoothing}}.
\end{equation}
These gradients partially cancel: one demands sharp boundaries, the other smooth transitions across slices. In our 2.5D design, the 2D backbone is frozen, so its weights receive \emph{only} the in-plane gradient during the first training stage. The 3D head's weights receive only the consistency gradient. This complete separation eliminates gradient conflict and allows each component to specialize fully.

\subsection{Fisher Information}

The Fisher information of the predicted probability map at boundary voxels satisfies:
\begin{equation}
I_{\mathrm{2D}}^{\mathrm{boundary}}(\theta) > I_{\mathrm{3D}}^{\mathrm{boundary}}(\theta),
\end{equation}
because the 2D network's sharp probability transitions yield large $|\partial \hat{p}_c / \partial \theta|$, while a 3D network's smoothed transitions yield smaller derivatives. At inter-slice voxels (requiring $z$-context), the reverse holds: $I_{\mathrm{3D}}^{\mathrm{context}} > I_{\mathrm{2D}}^{\mathrm{context}}$. Our 2.5D architecture captures both: the frozen 2D backbone retains maximal boundary Fisher information, while the 3D head contributes Fisher information at inter-slice transitions. By the Cram\'{e}r--Rao bound, the combined estimator achieves lower variance than either component alone.
